# Supplementary material for: AMOM: Adaptive Masking over Masking for Conditional Masked Language Model
Source: arXiv:2303.07457 source file (2023-03-13)
Supplement: Supplementary file 1 [file appendix.tex]

\newpage
\section{Additional Remarks of AMOM}
\label{app:method}
Figure~\ref{fig:amom_model} illustrates how our AMOM works during training, taken an example, when we train a sample pair from German ($X$ = \texttt{[Wir das das vollkonmen]}) to English ($Y$ = \texttt{[We totally accept it]}), we first adopt the original uniform masking strategy to divide $Y$ into $Y_{mask}$ and $Y_{obs}$, the result after uniform masking is denoted as $\hat{Y}$, then the tokens in $Y_{mask}$ (\texttt{[totally]} and \texttt{[accept]}) will be masked and we can compute the masking ratio of $Y$ and adopt the function $\varphi(\cdot)$ to decide the masking ratio of $X$, $\alpha=0.5$, $\varphi(\alpha)=0.2$. As a result, \texttt{[das]} in $X$ is masked, the result of adaptive $X$ masking of $X$ is denoted as $\hat{X}$. Then $\hat{X}$ and $\hat{Y}$ are passed through the encoder and decoder respectively to predict the masked tokens in $Y_{mask}$ using loss $L_{cmlm}$, here $Y_{mask}= \{\texttt{[totally]},\texttt{[accept]}\}$. After predicting the tokens in $Y_{mask}$ in the first training scheme (the result is denoted as $\hat{Y}_{mask}$, $\hat{Y}_{mask} = \{\texttt{[simply]}, \texttt{[accept]}\}$), we compute the correction ratio and adopt adaptive $Y$ masking strategy to decide the masking probability, as $\beta=0.5$, $\psi(\beta)=0.5$, then we will give the corresponding masking probability for tokens in $\hat{Y}_{mask}$ ($\psi(\beta)$) and $Y_{obs}$ ($1-\psi(\beta)$). As a result, \texttt{[We]} in $Y_{obs}$ and \texttt{[accept]} in $\hat{Y}_{mask}$ are newly masked, leading to a new subset of masked and unmasked tokens, denoted as $Y'_{mask}$ and  $Y'_{obs}$. The model then predicts tokens in $Y'_{mask}$ in the second training scheme using loss $L_{aday}$. Note that we use the model prediction (\texttt{[simply]}) rather than ground truth (\texttt{[totally]}) as newly part of $Y'_{obs}$ in the second training scheme to help reduce the problem of exposure bias.

\begin{figure*}[!htb] 
\centering
\includegraphics[scale=0.42]{LaTeX/PAPER/picture/amom.pdf}
\caption{A training example with adaptive masking over masking.}
\label{fig:amom_model} 
\end{figure*} 

We also compare our methods with two improvement methods~\cite{ghazvininejad2020semi,huang2022improving}, which also focus on releasing the gap between training and inference of original CMLM and improving the ability of refinements. 
SMART~\cite{ghazvininejad2020semi} and CMLMC~\cite{huang2022improving} both introduce a correction mechanism, which aims to simultaneously correct some specific tokens and generate the masked tokens in each iteration during inference. To realize this purpose, they design particular training 
schedules. In SMART, it first applies the decoder to generate predictions of the whole sentence depending on $\{X, Y_{obs}\}$, then adopts a uniform masking strategy over these predictions. It applies the decoder to learn to self-correct the reserved unmasked tokens while simultaneously reconstructing newly masked tokens.
However, CMLMC points out that this procedure may not be optimal.
They argue that the most significant mistakes are made during the first iteration where the tokens are predicted from the fully masked sentence with no ground truth. In the training process of SMART, it does self-correction on the results generated with some ground truth tokens $Y_{obs}$ as input. Thus they design a better procedure to teach the model to learn self-correction. CMLMC replaces some tokens in $Y_{obs}$ with the results predicted from a fully masked sentence and applies the decoder to self-correct these replaced tokens. 
% Although this correction mechanism truly improves the generation quality,
During inference\footnote{Introduction of inference schedule can be found in section Methodology. If you want more details, see the original CMLM paper.}, these two methods improve the generation quality by adding a correction mechanism, thus enhancing the ability to refine unmasked tokens rather than to predict the masked tokens depending on different unmasked tokens. 
In contrast, our AMOM enhances the ability to predict the masked tokens over different masking conditions in multiple iterations by introducing adaptive masking over masking strategy, where adaptive $X$ masking aims to construct encoder input with a specific masking ratio coordinated with the masking ratio of $Y$ and adaptive $Y$ masking aims to capture the effects of masking ratio changes by adding a second adaptive masking scheme during training. They both urge the model to focus more on the target information $Y_{obs}$ and improve the ability to predict the masked tokens conditional on different unmasked tokens in multiple inference iterations.

Generally speaking, the original inference algorithm (mask predicted) in CMLM keeps masking and predicting specific tokens in multiple inference iterations without operation on unmasked tokens. SMART and CMLMC change the inference algorithm to match their self-correction mechanism, where the unmasked tokens will also be refined during every iteration. Our AMOM adopts the original mask predicted inference algorithm. Notice that the tokens which are predicted ($Y_{mask}$) and depended on ($Y_{obs}$) in each inference iteration are entirely different. We assume that the CMLM can not capture these changes in various inference iterations with its original training scheme. Although different masking scenes may be reflected by one specific uniform masking scene in training, $X$ is fixed (without any operation on $X$) in different masking scenes, the model may ignore the difference of each masking scene due to the strong condition of $X$, then the model can not learn useful information of changes in $Y_{mask}$ and $Y_{obs}$, which is the motivation of our adaptive $X$ masking strategy.
Moreover, the number of masked tokens in each iteration with low confidence will gradually decrease, and the unmasked tokens relied on to make predictions will change relevantly during inference. However,  only one-step uniform masking is adopted, leading to a gap during training, which motivates our adaptive $Y$ masking strategy.

\section{More Details of AMOM}
\subsection{Early Analytical Experiments}
As mentioned above, the difference of each masking scene during training may be ignored with the strong condition of $X$ if without any operation on $X$. Table~\ref{tab:mask_x} shows that introducing some masking strategy on $X$ significantly improves the performance in Iter.10. In this section, we explore the performance in Iter.1, and the results of introducing some masking strategy on $Y_{obs}$, which explains the necessity of Adaptive $X$ masking from another angle. Table~\ref{tab:masking_X_more} shows the results of different
masking strategies on $X$ and $Y_{obs}$. We can observe: 1) With masking on $X$, the BLEU score in Iter.1 drops a little (28.18 vs. 27.46 / 26.40 / 27.15), but with more iterations, the BLEU score increases in Iter.10 (33.87 vs. 34.10 / 34.18 / 34.07), and the fixed masking strategy may be not optimal for under some specific scenes, for example, Bleu in Iter.1 drops seriously, which is caused by lacked information of $X$; 2) With masking on $Y_{obs}$, the BLEU score in Iter.1 increases gradually (28.18 vs. 28.23 / 28.36 / 28.58) as the masking ratio increases, but there is no great improvement of the BLEU score in Iter.10 (33.87 vs. 33.54). This indicates that the BLEU score in Iter.1 is more related to $X$ (source information) and in later iterations (refinements) is related to $Y_{obs}$ (target information). Also, the improvements from Iter.1 to Iter.10 are more remarkable with $X$ masking strategy, but decline with $Y_{obs}$ masking, which also supports our assumption that information from $Y$ is more important for refinements. As a result, it is necessary to capture the changes of $Y$ during training by adaptive $Y$ masking strategy.

\begin{table}[!htb]
\centering
\small
\scalebox{0.94}{
\begin{tabular}{lccc}
\toprule
\textbf{Method} & \textbf{Iter.1} & \textbf{Iter.10} & \textbf{$\Delta$ BLEU} \\
\midrule
CMLM & 28.18 & 33.87 & 5.69\\
\midrule
\textbf{Masking on $X$}\\
Fixed (0.1) & 27.46 & 34.10 & 6.64 \\
Fixed (0.2) & 26.40 & 34.18 & 7.74\\
Fixed (0.3) & 25.23 & 34.07 & 8.84 \\
\midrule
\textbf{Masking on $Y_{obs}$}\\
Fixed (0.1) & 28.23 & 33.64 & 5.41\\
Fixed (0.2) & 28.36 & 33.68 & 5.36\\
Fixed (0.3) & 28.58 & 33.54 & 4.96\\
\bottomrule
\end{tabular}}
\caption{BLEU scores of fixed masking on $X$ and $Y_{obs}$.}
\label{tab:masking_X_more}
\end{table}

\subsection{Experimental Settings}
We list the detailed training settings here.
\begin{table}[!htb]
\centering
\small
\resizebox{0.95\columnwidth}{!}{
\begin{tabular}{lccccc}
\toprule
\textbf{Datasets} & WMT'14 & WMT'16 & IWSLT'14 & XSUM & Code \\
\midrule
learning rate & 7e-4 & 5e-4 & 5e-4 & 1e-4 & 5e-5\\
warmup & 40k & 10k & 10k & 10k & 4k\\
dropout & 0.1 & 0.3 & 0.3 & 0.1 & 0.1  \\
GPU & 8 GTX 3090 & 4 GTX 3090 & 1 GTX 3090 & 4 RTX A5000 & 2 RTX A5000\\
tokens/GPU & 8192 & 8192 & 8192 & 4096 &8192 \\
max-update & 300k & 300k & 300k & 180k & 300k \\
update-freq & 2 & 1 & 1 & 2 & 1 \\
\bottomrule
\end{tabular}}
\caption{AMOM training hyper-parameters.}
\label{tab:settings}
\end{table}

\subsection{Mapping Function }
We plot the curves of mapping functions here. Also, we further explore the effects of adaptive $X$ masking ratio ranges on WMT RO$\to$EN dataset in Table~\ref{tab:ratioadax}, results show that a simple and reasonable masking ratio range can significantly improve the performance, since we select (0.3,0.1) for all datasets, we see a universal improvement, performance can be further improved through more granular search. 

\begin{figure}[!htb]
\centering
\subfigure[Encoder($a=0.3,b=0.1$)]{
\includegraphics[scale=0.22]{LaTeX/PAPER/picture/ada_x.pdf}
\label{fig:adax_map}
}
\subfigure[Decoder($a=0.2,b=0.8$)]{
\includegraphics[scale=0.22]{LaTeX/PAPER/picture/ada_y.pdf}
\label{fig:aday_map}
}
\captionof{figure}{The curves of different $\varphi$ function (x-axis denotes \\the $\alpha_{dec} $ and $\beta$ for Encoder and Decoder respectively).}
\label{fig:mapping function}
\end{figure}

\begin{table}[htb]
\centering
\small
\resizebox{0.9\columnwidth}{!}{
\begin{tabular}{lcccc}
\toprule
Ratio & None & (0.3,0.1) &	(0.3,0.2)&	(0.4,0.2)\\
\midrule
BLEU &	33.56&	34.32&	34.35&	34.27\\
\midrule
Ratio &	(0.4,0.15)&	(0.35,0.15)& (0.35,0.1)&	(0.1,0.3) \\
\midrule
BLEU &	34.24	&34.46&	\textbf{34.38}&	33.72 \\
\bottomrule
\end{tabular}}
\caption{Results of $X$ masking for WMT RO-EN dataset.}
\label{tab:ratioadax}
\end{table}

We also give a brief insight for choosing the masking ratio limits (0.8,0.2) of our adaptive $Y$ masking
strategy. 
Once $m$ tokens in $Y$ are masked in the first uniform masking, the model generate tokens in $Y_{mask}$, denoted as $\hat{Y}_{mask}$, $n = |\hat{Y}_{mask}!=Y_{mask}|$, denoted as the number of incorrect tokens,
then $\beta = \frac{n}{m}$, denoted as error rate of $Y_{mask}$, the each token in $\hat{Y}_{mask}$ has a possibility of $p$ to be masked and $p$ is a function of $\beta$ mentioned in Section Methodology.
Suppose the length of $Y$ is $L$, then the expectation of the number of tokens predicted incorrectly in 
$\hat{Y}_{mask}$ to be masked in the second adaptive masking step is $E_{num}= n * p = m * \beta * p $, Since $m$ uniform distribution of $L$, $E_{num} = E_{m} * \beta *p = 0.5 * L * \beta *p$.
In our adaptive $Y$ masking, $p = 0.6 (1 - \beta) + 0.2$, then the expectation of the ratio of tokens predicted incorrectly in $Y$ is $E_{r} = \frac{E_{num}}{L} = 0.5* \beta * (0.6 (1 - \beta) + 0.2) = 0.4 \beta - 0.3 \beta^2 $, the correct ratio $\lambda = 1 - \beta$, then $E_{r} = -0.3 \lambda^2 + 0.2 \lambda +0.1 $. As a result, when the accuracy is between 0\% and 66\%, $E_{r}$ is stable at 10\% to 13\%, indicating the current iteration is not reliable, and the model will be hard to choose correct tokens by confidence, when the accuracy is between 66\% and 100\%, the accuracy is already high, $E_{r}$ is a bit lower. At this time, model can perform well in current iteration and other tokens predicted in the previous iteration with low confidence will be masked, our adaptive $Y$ masking matches the inference schedule.

\section{More Comparison between AMOM and CMLM}
\subsection{Effective of adaptive masking}
We investigate the effectiveness of each adaptive masking strategy for different iteration steps based on CMLM.
In Table~\ref{tab:ablation}, we show the BELU scores of each Adaptive $X$ Masking (Ada-$X$), Adaptive $Y$ Masking (Ada-$Y$), and Adaptive Masking Over Masking (AMOM) experiment.
With the Adaptive Masking strategy, the model can outperform the baseline in each iteration step. That demonstrates that dynamic masking is beneficial for the model to learn robust representation.
Finally, AMOM achieved the best BLEU score of $34.84$. It outperforms Adaptive $X$ or $Y$ Masking strategy, proving the two-stage masking is more effective and obtains superior performances at each iteration step.
\begin{table}[!htb]
\centering
\scalebox{0.9}{
\begin{tabular}{l c c c }
\toprule
Method & Iter.1 & Iter.4 & Iter.10\\
\midrule
CMLM & 27.64 & 33.20 &33.87 \\
+ Ada-$X$ & 27.15 & 33.62 &34.48  \\
+ Ada-$Y$ & 28.88 & 33.45 &33.93 \\
+ AMOM &27.44 &\textbf{33.90} &\textbf{34.84}\\
\bottomrule
\end{tabular}}
\captionof{table}{Results for each component of the AMOM.}
\label{tab:ablation}
\end{table}

\begin{table}[!htb]
\centering
\scalebox{0.65}{
\centering
    \begin{tabular}{l c | l c}
    \toprule
    \textbf{Masking Strategy} & \textbf{BLEU} & \textbf{Masking Strategy} & \textbf{BLEU} \\
    \midrule
    Adaptive (Ours) & \textbf{34.84} &Uniform  & 34.53 
     \\
    \midrule
    Adaptive + same ratio & 34.65 &
    Uniform + same ratio & 34.36\\
    \midrule
    Adaptive + 3 step & 34.50& 
    Uniform + 3 step & 34.16\\
    \midrule
    Adaptive + exposure bias  & 34.79 &
    Uniform + exposure bias & 34.48\\
    \midrule
    Adaptive + confidence-based  & 33.85 &
    Uniform + confidence-based & 33.74\\
    \bottomrule
    \end{tabular}}
\caption{BLEU scores of different masking constraints.}
\label{tab:com1}
\end{table}

\subsection{Training Strategies }
Table~\ref{tab:adaptve Y} presents the results of the adaptive $Y$ masking strategy with various constraints to better show the effectiveness of adaptive $Y$ masking compared with the original masking scheme in CMLM. We also conduct experiments with uniform masking, Table~\ref{tab:com1} presents these results; we can obverse that adopting the adaptive $Y$ masking strategy in the second training step outperforms uniform masking with the same constraint, which further verifies the necessity and effectiveness of the two-step adaptive masking strategy.

\subsection{Effects of Iterations}
We plot the BLEU scores of 10 iterations here to show the effectiveness of AMOM compared to the original CMLM for improving the refinements, we observe that AMOM also gains rapid improvements with more iterations.
Besides, we also show the results of different iterations in the summarization task in Table~\ref{tab:xsum_new}, we also find with more iterations, AMOM gains more significant improvement (2.09$\uparrow$ on ROUGE-1, 2.09$\uparrow$ on ROUGE-2 and 0.96$\uparrow$ on ROUGE-L), but CMLM achieves little improvements.

\begin{figure}[h]
\centering
\subfigure[EN$\to$RO]{
\includegraphics[scale=0.259]{LaTeX/PAPER/picture/en_ro_new.pdf}
}
\subfigure[RO$\to$EN]{
\includegraphics[scale=0.259]{LaTeX/PAPER/picture/ro_en_new.pdf}
}
\subfigure[EN$\to$DE]{
\includegraphics[scale=0.3]{LaTeX/PAPER/picture/en-de.pdf}
}
\subfigure[DE$\to$EN]{
\includegraphics[scale=0.3]{LaTeX/PAPER/picture/de-en.pdf}
}
\captionof{figure}{The BLEU scores for Iter.1-10 on WMT'16 EN-RO and WMT' 14 EN-DE translation tasks.}
\label{fig:diff_step}
\end{figure}

\begin{table}[h]
\centering
\scalebox{0.85}{
\begin{tabular}{l c c c c }
\toprule
\textbf{Model} & Iter. & ROUGE-1 &ROUGE-2 &ROUGE-L\\
\midrule
\multirow{3}{*}{CMLM}  & 4 & 25.90 & 5.68 & 20.63 \\
& 7 & 25.78 & 6.07 & 20.49 \\
 & 10& 25.80 & 6.31 & 20.45	\\
\multirow{2}{*}{AMOM} & 4 & 29.50 & 7.21 & 23.94 \\
& 7 & 30.93 & 8.69 & 24.69 \\
 & 10 & \textbf{31.59} & \textbf{9.30} & \textbf{24.98}	 \\
\bottomrule
\end{tabular}}
\caption{Results on XSUM for the summarization task.}
\label{tab:xsum_new}
\end{table}

% \begin{table}[!htb]
% \centering
% \scalebox{0.85}{
% \begin{tabular}{l c c c c }
% \toprule
% \textbf{Model} & Iter. & ROUGE-1 &ROUGE-2 &ROUGE-L\\
% \midrule
% \multirow{3}{*}{CMLM}  & 4 & 25.90 & 5.68 & 20.63 \\
% & 7 & 25.78 & 6.07 & 20.49 \\
%  & 10& 25.80 & 6.31 & 20.45	\\
% \multirow{2}{*}{AMOM} & 4 & 29.50 & 7.21 & 23.94 \\
% & 7 & 30.93 & 8.69 & 24.69 \\
%  & 10 & \textbf{31.59} & \textbf{9.30} & \textbf{24.98}	 \\
% \bottomrule
% \end{tabular}}
% \caption{Results on XSUM for the summarization task.}
% \label{tab:xsum_new}
% \end{table}

\begin{table*}[htb!]
\centering
\scalebox{0.89}{
\centering
\begin{tabular}{l c c c c c c c c c}
\toprule
\multirow{2}{*}{\textbf{Model}} &  \multirow{2}{*}{\textbf{Iterations}} & \multicolumn{2}{c}{\textbf{WMT16}} & \multicolumn{2}{c}{\textbf{WMT14}}  \\
& & \textbf{EN$\to$RO} & \textbf{RO$\to$EN} & \textbf{EN$\to$DE} & \textbf{DE$\to$EN} & \\
\midrule
Transformer w/ Com. &$N$ & 34.23(34.0) & 34.28(34.0) & 28.41(28.2) & 32.28(31.9)\\
\midrule
\multirow{2}{*}{\textbf{CMLM}}
  & 4 & 32.53 & 33.23& 25.94& 29.90\\
  & 10 & 33.03 & 33.31 & 27.03& 30.53\\
\multirow{2}{*}{\textbf{w/ Com.}}
  & 4 & 32.60(32.5) & 33.15(33.2) & 25.79 (25.1)& 29.95 (29.5)\\
  & 10 & 33.46(33.0) & 33.83(33.7) & 27.21 (26.5)& 31.03 (30.5) \\
\midrule
\multirow{2}{*}{\textbf{AMOM}}
  & 4 & 33.69(33.6) & 34.34(34.3) & 26.35 (25.8) & 30.22(29.8) \\
  & 10 & 34.10(34.0) & 34.89(34.8) & 27.80 (27.2) & 31.32(30.8) \\
\multirow{2}{*}{\textbf{w/ Com.}}
  & 4 & 33.32(33.2) & 33.74(33.8) & 25.04 (24.4) & 29.47(29.1)\\
  & 10 & 34.62(34.4) & 34.82(34.9) & 27.57 (26.9) & 31.67(31.2) \\
\bottomrule
\end{tabular}}
\caption{Results trained on only-distilled and combined data, Com. denotes training with combining the raw and distilled data. Numbers in the bracket denotes SacreBleu.}
\label{tab:rawdata}
\end{table*}

\begin{figure}[!htb]
\centering
\subfigure[Train loss]{
\includegraphics[scale=0.11]{LaTeX/PAPER/picture/de_en_train1.pdf}
}
\subfigure[Valid loss]{
\includegraphics[scale=0.11]{LaTeX/PAPER/picture/de_en_valid1.pdf}
}
\subfigure[Valid BLEU]{
\includegraphics[scale=0.11]{LaTeX/PAPER/picture/de_en_bleu.pdf}
}
\subfigure[RO-EN]{
\includegraphics[scale=0.11]{LaTeX/PAPER/picture/ro_en.pdf}
}
\subfigure[EN-RO]{
\includegraphics[scale=0.11]{LaTeX/PAPER/picture/en_ro.pdf}
}
\subfigure[EN-DE]{
\includegraphics[scale=0.11]{LaTeX/PAPER/picture/en_de.pdf}
}
\captionof{figure}{Curves along with model training.}
\label{fig:trainingbleu}
\end{figure}

\begin{figure}[!htb]
\centering
\subfigure[Machine translation]{
\includegraphics[scale=0.45]{LaTeX/PAPER/picture/example1.pdf}
}
\subfigure[Summarization]{
\includegraphics[scale=0.45]{LaTeX/PAPER/picture/example3.pdf}
}
\subfigure[Code generation]{
\includegraphics[scale=0.45]{LaTeX/PAPER/picture/example2.pdf}
}
\captionof{figure}{Generation examples of different tasks.}
\label{fig:example}
\end{figure}

\subsection{Effects of Datasets}
Since we combine the raw and distilled data as our final training datasets for WMT tasks mentioned above, which is introduced in \cite{ding2020understanding}, we also train AMOM on only-distilled data, see Table~\ref{tab:rawdata}. Besides, we also report the SacreBLEU~\footnote{\url{https://github.com/mjpost/sacrebleu}} to make a further comparison.
For CMLM baseline, we report the number in their original paper. Results show that CMLM training with combined data outperforms vanilla CMLM in all datasets, which has been studied in \cite{ding2020understanding}. AMOM outperforms vanilla CMLM both trained with only-distilled and combined data in all datasets, with about 1 BLEU improvement on WMT14 EN-RO datasets and 0.6 BLEU improvement on WMT14 EN-DE datasets. The results are consistent for SacreBleu, which also shows the effectiveness of AMOM. Need to notice that AMOM outperforms its AT counterpart on WMT EN-RO datasets. However, training with only-distilled data outperforms that with combined data in WMT14 EN$\to$DE and WMT16 RO$\to$EN datasets.

\subsection{Training Process}

Since we change the training scheme, we explore the effects of different aspects during training (e.g., the changes in train loss, valid loss and valid BLEU). Hence, we plot the curves of train/valid loss and valid BLEU of the IWSLT DE$\to$EN dataset along with the training update number for our AMOM and original CMLM in Figure~\ref{fig:trainingbleu}. We can observe: 1) Along with the training, the training loss of CMLM is always lower than AMOM, which is contrary to the comparison of valid loss. This indicates that the training scheme in CMLM may not be optimal, and CMLM will become over-fitting seriously in the middle and late stages of training. The gap between the train and valid loss of CMLM is large. 2) As shown in the curve of valid BLEU of Iter.10, AMOM outperforms original CMLM significantly throughout the training process. Besides, this also reflects a gap between the BLEU score of Iter.10 and train/valid loss. The results of train/valid loss may not be able to reflect the performance of generated tokens with multiple iterations. This also indicates the limitation of the original CMLM training scheme.
Besides, although AMOM is slower than CMLM during training since they need to forward the model twice, we suppose that the training efficiency is more effective than CMLM, see Figure~\ref{fig:trainingbleu}.(c), AMOM can achieve the best BLEU score of the vinilla CMLM at around 70k update number, only 1/4 of the whole training process, indicating that although AMOM is slow(around 1.8 times than CMLM) during training, AMOM is also more effective than CMLM in general, we also show two other language pairs in Figure~\ref{fig:trainingbleu}, results are consistent. Besides, we compare the training process with only-distilled data and combined data, it seems training on the only-distilled data is better than that on the combined data on the WMT14 EN$\to$DE dataset.

Besides, we give some quantitative analysis of training efficiency. Each training step of AMOM indeed costs more time than the vanilla CMLM model (e.g., each training epoch of CMLM and AMOM on WMT RO-EN dataset will takes around 133.4 seconds and 249.4 seconds (1.9 times over CMLM) on 4 RTX A5000 GPU cards, respectively). But the overall convergence speed of AMOM is not so slow compared with CMLM. For instance, the CMLM model is converged on WMT RO-EN dataset with around 3.65 hours while AMOM only takes around 2.35 hours longer (+ 70\% training time), which is worthwhile, especially considering the universal performance improvement. 
Besides, the performance of our AMOM grows more rapidly than CMLM, i.e., our method can achieve the same or better performance with less training time than CMLM. Take the experimental results (BLEU score) on for example, Table~\ref{tab:validbleuduringtraining} shows the valid BLEU score along with the training time, we can observe that our method can achieve better performance after 3 hours training (which is less the convergence time of CMLM).

\begin{table}[htb]
\centering
\small
\resizebox{0.95\columnwidth}{!}{
\begin{tabular}{lccccccc}
\toprule
Time (hours)	& 1h &	2h &	3h &	5h	& 10h& 	15h	 &20h  \\
\midrule
AMOM &	17.83&	31.45&	34.03&	34.91	&35.92&	36.34&	36.45 \\
CMLM &	29.65&	32.91&	33.99&	34.63	&35.09	&35.29&	- \\
\bottomrule
\end{tabular}}
\caption{Valid BLEU scores along with the training time.}
\label{tab:validbleuduringtraining}
\end{table}

\subsection{Generation Examples}
We give some generation examples for better comparing AMOM and CMLM on generation quality, since we verify AMOM at three different tasks, we all give an example to analyze the difference between CMLM and AMOM. We can observe that AMOM can better handle the details of the sentence and make the sentence more fluent.
